# Supplementary material for: Automatic Layout Planning for Visually-Rich Documents with Instruction-Following Models
Source: arXiv:2404.15271 source file (2024-04-23)
Supplement: Supplementary file 1 [file A.tex]

\todo{data preprocessing, remove smaller than 5\% etc}

\todo{model details}

\todo{error analysis}

\todo{prompts for gpt4}
